# Supplementary material for: InterCode: Standardizing and Benchmarking Interactive Coding with Execution Feedback
Source: arXiv:2306.14898 source file (2023-10-30)
Supplement: Supplementary file 1 [file misc.tex]

\section{Data Collection Risks}
\label{appx:misc:data_collection_cklist}

The transformations performed to the NL2Bash~\cite{lin-etal-2018-nl2bash} and Spider~\cite{yu-etal-2018-spider} datasets generally involve removing instructions with gold commands that are not supported by the given task environment, grounding instructions and commands to the environment, and removing unnecessary fields provided by the original dataset from the version adapted to \benchmark{}. Given this technically based re-purposing of the dataset, we believe that these changes do not introduce any new risks that were not present in the original dataset.

The human trajectories discussed in \S~\ref{appx:experiments:human_perf} are a small-scale study that again, was performed by the authors to gauge the performance gap between large language models and experts. These trajectories are available in the linked repository and created from the same logging mechanism that was used for the experiments performed on base models with different prompting strategies. The trajectories do not capture any personal information. With that said, given that these trajectories are the product of a small set of individuals, the problem-solving strategy reflected across trajectories may be biased towards some techniques and lean less heavily on others. Approaches that attempt to leverage human feedback and guidance toward training or tuning code models and language models should be founded on more extensive and thorough human demonstration data collection.

\section{Potential Societal Impacts \& Limitations}
\label{appx:misc:potential_impacts}

\benchmark{}'s goal of formulating tasks to advance the development decision-making and code agents is an exciting research direction that also warrants concerns about safety and fairness.

\textbf{Coverage of languages.} The \benchmark{} codebase currently features two tasks with Bash and SQL programming languages as action spaces. We plan to expand the number of \benchmark{} based tasks to cover more programming languages as further demonstrations of the \texttt{\benchmark{}Env}'s utility along with improving \benchmark{}'s ease of use for practitioners interested in \benchmark{} as a training platform. As well as programming languages, additional ongoing work also aims to feature more datasets, task environments, and types of tasks.

\textbf{Limitations of the CTF task.} The Capture the Flag toy dataset showcases \benchmark{}'s serviceability for developing novel tasks with new code understanding challenges that can easily be used for training and evaluating models. With that said, this demonstration currently only has four task instances. We hope to put forth a more thorough examination of the Capture the Flag task's challenges, provide a clearer picture of the performance of existing models on this task, and release a more comprehensive dataset.

\textbf{Training agents with \benchmark{}.} While \benchmark{} in its current state can be used as a training platform for decision-making code agents, the existing codebase does not currently include any examples of training code that uses \benchmark{} in this manner. This is a direction we are interested in pursuing shortly. The \benchmark{} task formulation and usage of the Gym API naturally lends itself to use for creating decision-making agents that can leverage techniques such as reinforcement learning or imitation learning.

\textbf{Safety of developing code agents.} \benchmark{}'s use of Docker containers ensures the safe execution of commands in a realistic simulated task environment. With this said, the Bash and SQL \benchmark{} environments currently do not explicitly impose any strict limitations on the action space. While the execution of irreversibly detrimental commands is mitigated by Docker, a direct sim-to-real transfer of an \benchmark{}-trained agent to a real system may put the system at risk. To combat this, the \texttt{\benchmark{}Env} interface allows task designers to add their own execution logic that can provide guardrails on model behavior and define an allow-list of permissible commands to eliminate the risk of potentially disastrous commands.
